# Supplementary material for: Proof of Federated Training: Accountable Cross-Network Model Training and Inference
Source: arXiv:2204.06919 source file (2022-04-14)
Supplement: Supplementary file 1 [file 08.Appendix.tex]

\begin{appendices}

\section{Pilot Study} \label{sec:app-A}
The initial study conducted in Section \ref{sec:pilot} 

\end{appendices}
